# Supplementary material for: Meta-Prompting for Automating Zero-shot Visual Recognition with LLMs
Source: arXiv:2403.11755 source file (2024-08-07)
Supplement: Supplementary file 1 [file erratum.tex]

\section{Erratum}
\label{sec:supp:erratum}

In the main manuscript Table $4$, the \method accuracy for CIFAR-100~\cite{cifar} should actually be $66.3\%$ (consistent with the results reported in Table $1$ of the main manuscript for the same ViT-B/32 backbone from CLIP~\cite{clip}), which is higher than the $64.4\%$ that we reported in Table $4$ by mistake. %Sorry!
