# Supplementary material for: Meta-Prompting for Automating Zero-shot Visual Recognition with LLMs
Source: arXiv:2403.11755 source file (2024-08-07)
Supplement: Supplementary file 2 [file truncating_prompts.tex]

\section{Truncating VLM prompts}
\label{sec:supp:truncating_VLM_prompts}

% \begin{table*}[]
%     \centering
%     % \resizebox{0.7\textwidth}{!}{
%         \setlength{\tabcolsep}{10pt}

%     \begin{tabular}{c|cccc}
%     \toprule
%          &  GPT & Mixtral & GPT - CLS & Mixtral - CLS\\
%         \midrule
%         \midrule
%        ViT-B32 & {62.9} & {62.4} & {44.9} & {24.0} \\
% ViT-B16 & {66.7} & {66.4} & {48.5} & {25.5} \\
% ViT-L14 & {73.4} & {72.5} & {55.2} & {28.4} \\
%         \bottomrule
%         \bottomrule
%     \end{tabular}
%     % }
%     \caption{Caption}
%     \label{tab:my_label}
% \end{table*}
\begin{table}[t!]
\small
        \setlength{\tabcolsep}{8pt}

    \centering
    \begin{tabular}{l|cc|cc}
\toprule

 & GPT & Mixtral & Truncated GPT & Truncated Mixtral \\
\midrule
\midrule

ViT-B/32 & {62.9} & {62.4} & {56.2} & {55.5} \\
ViT-B/16 & {66.7} & {66.4} & {59.8} & {60.2} \\
ViT-L/14 & {73.4} & {72.5} & {67.6} & {67.1} \\
\bottomrule
\bottomrule

\end{tabular}
    \caption{Comparison of mean top-1 accuracy (\%) over 20 datasets obtained by using the complete description set for \method (first two columns) and truncating the text descriptions with a fixed window.}
    \label{tab:trunate-descriptions}
\end{table}
% \begin{tabular}{lrrr}
% \toprule
%  & GPT & Mixtral & Truncated GPT \\
% \midrule
% ViT-B_32 & {62.9} & {62.4} & {56.2} \\
% ViT-B_16 & {66.7} & {66.4} & {59.8} \\
% ViT-L_14 & {73.4} & {72.5} & {67.6} \\
% \bottomrule
% \end{tabular}

To explore the effect of \emph{descriptiveness} of our LLM-generated VLM prompts, we design an experiment where we truncate the prompts for each class with a fixed window size, randomly chosen between $50\%\to70\%$ for each description (VLM prompt) but we take care that the class name is not removed if it was included in the original description. 
These results are provided in Table~\ref{tab:trunate-descriptions}, where we report the average of $5$ random runs when truncating the descriptions. 
These results indicate that the CLIP text encoder responds well to syntactically correct (and descriptive) sentences, further highlighting the reason why our \method performs better than Waffle~\cite{waffle}, which adds random descriptors to high-level concepts.
