# Supplementary material for: Meta-Prompting for Automating Zero-shot Visual Recognition with LLMs
Source: arXiv:2403.11755 source file (2024-08-07)
Supplement: Supplementary file 3 [file incontext_dataset_ablation.tex]

\begin{table}[t!]
    \centering
                    \setlength{\tabcolsep}{10pt}

    \begin{tabular}{llc}
    \toprule
         in-context dataset & target dataset &top-1 (\%)\\
         \midrule
         \midrule
        Flowers & DTD&52.0\\
                EuroSAT & DTD &50.8\\

        CUBS & DTD&51.8\\
         \midrule

         Flowers & EuroSAT&54.5\\
         CUBS &EuroSAT&54.4\\
                          DTD & EuroSAT&55.6\\

         \bottomrule
         \bottomrule
    \end{tabular}
    \caption{Top-1 accuracy (\%) with ViT-B/32~\cite{clip} while using different datasets as the in-context example dataset in the stage-1 of \method (meta-prompting).}
    \label{tab:in_context_dataset_ablation}
\end{table}
